# Supplementary material for: Pleiotropy enables specific and accurate signaling in the presence of ligand cross talk
Source: arXiv:1911.05895 ancillary file (2021-04-02)
Supplement: Supplementary file 1 [file Supplementary-final.pdf]

# Supplementary Material for "Effects of cross-talk and pleiotropy on the specificity and accuracy of receptor signaling"

*Code implementing the analysis, simulations, and plotting is available at https://github.com/uoftbiophysics/cellsignalling

## Contents

Section A: Calculating the moments of the output variables ........ 1
*General formalism* ........ 1
*Model 1 - Non-pleiotropic receptor* ........ 1
*Model 2 - Single state pleiotropic receptor* ........ 2
*Model 3 - Multi-state pleiotropic receptor* ........ 2
Section B: Obtaining Maximum Likelihood Estimates of $c$ and $k_{\mathrm{off}}$ ........ 3
*MLE for Model 1* ........ 4
*MLE for Model 2* ........ 5
*MLE for Model 3* ........ 6
Section C: Accuracy of the estimators ........ 6
*Full expression for the Fisher Information Matrix* ........ 6
*General formalism* ........ 7
*Estimation Error for Model 2* ........ 8
*Estimation Error for Model 3* ........ 8
*Comparison of Heuristic Covariance to the full CRLB* ........ 8
Section D: Alternative calculation of the moments of the distribution of $n$ and $m$ ........ 9
*Moments of the distribution of* $n$ ........ 9
*Moments of the distribution of* $m$ ........ 11
Section E: Long time distribution well-approximated by a Normal distribution ........ 12
Section F: Bayesian framework, effects of the prior ........ 13

# Section A: Calculating the moments of the output variables

In the main text we consider several schemes of receptor kinetics. They are referred to within the Supplemental Material (SM) by

- Model 1: Single state non-pleiotropic receptor
- Model 2: Single state pleiotropic receptor
- Model 3: Multi-state pleiotropic receptor

## *General formalism*

In this section, we present the general form of the generating function formalism. Specifically, for the case of two output molecules $n$ and $m$, the state of the system is described by the master equation for the probability distribution $P_i^{n,m}(t)$. The corresponding generating function is $G_i(s,q,t) = \sum_{n,m=0}^{\infty} s^n\, q^m P_i^{n,m}(t)$. Vectorizing the generating function as $\mathbf{G}(s,q,t) = \begin{bmatrix} G_0 \\ G_1 \end{bmatrix}$, its dynamics are described by

$$\frac{\partial \mathbf{G}(s,q,t)}{\partial t} = \mathbf{M}(s,q)\mathbf{G}(s,q,t) \tag{S1}$$

where $\mathbf{M}$ is the transition matrix derived from the master equation, as in Eq. (2) of the main text.

Throughout the text we assume that the initial state of the receptor is the steady state occupancy, $\mathbf{P}^{\text{ss}}$, which allows us to write $G_i(s=1, q=1, t=0) = P_i^{ss}$. This analysis can be repeated for arbitrary initial conditions. In the long time limit, $k_{\text{off}}t \gg 1$ , the choice of initial condition does not alter our results (see next section).

Moments of the variables $n$ and $m$ can be derived from derivatives of $\mathbf{G}(s,q,t)$ with respect to $s$ and $q$ as in the main text [93]. For each model we considered, our moment expressions were validated using Gillespie simulation of the associated master equations (not shown).

## *Model 1 - Non-pleiotropic receptor*

With the initial condition outlined above, the generating function approach gives the following expression for $G(s,t) = G_0(s,t) + G_1(s,t)$:

$$G(s,t) = e^{-\frac{1}{2}\left(\sqrt{A}+k_{\text{off}}+ck_{\text{on}}+k_p(1-s)\right)t}(\sqrt{A}\left(1+e^{\sqrt{A}t}\right)(k_{\text{off}}+ck_{\text{on}}) + \left(-1+e^{\sqrt{A}t}\right)\left(k_{\text{off}}^2+ck_{\text{on}}\left(ck_{\text{on}}+k_p(-1+s)\right)+k_{\text{off}}\left(2ck_{\text{on}}+k_p(1-s)\right)\right)) \tag{S2}$$

where $A = {k_{\text{off}}}^2 + \left(ck_{\text{on}} + k_p(-1+s)\right)^2 + 2k_{\text{off}}\left(ck_{\text{on}} + k_p(1-s)\right)$. From this expression we derive the mean of $n$ shown in the main text (Eq. (3)), and variance

$$\langle \delta n^2 \rangle = \frac{k_p t x}{1+x} + \frac{2\,k_p^2 t x}{k_{\text{off}}(1+x)^3}\left(1 + \frac{e^{-t\,k_{\text{off}}(1+x)} - 1}{t\,k_{\text{off}}(1+x)}\right), \tag{S3}$$

where $x = ck_{\text{on}}/k_{\text{off}}$. This reduces to Eq. (3) of the main text for $k_{\text{off}}\,t \gg 1$.

## *Model 2 - Single state pleiotropic receptor*

The generating function transition matrix for Model 2 is

$$\mathbf{M}(\mathrm{s},\mathrm{q})=\begin{pmatrix}-k_{\mathrm{on}}c & k_{\mathrm{off}}\\ k_{\mathrm{on}}cq & -k_{\mathrm{off}}+k_p(s-1)\end{pmatrix}\tag{S4}$$

Using the generating function method, the variance and the covariance of the products $n$ and $m$, in the long time limit, are given in the main text (Eq. (7)).

## *Model 3 - Multi-state pleiotropic receptor*

The steady state receptor occupancies for the kinetic proofreading model with $k_f(k_{\mathrm{off}})=\frac{\alpha}{k_{\mathrm{off}}}$ are: $P_0^{ss}=\frac{1}{1+x_1+x_2}$, $P_1^{ss}=\frac{k_{\mathrm{off},1}^2x_1}{(1+x_1+x_2)(k_{\mathrm{off},1}^2+\alpha)}$, $P_2^{ss}=\frac{x_1\alpha}{(1+x_1+x_2)(k_{\mathrm{off},1}^2+\alpha)}$, $P_3^{ss}=\frac{k_{\mathrm{off},2}^2x_2}{(1+x_1+x_2)(k_{\mathrm{off},2}^2+\alpha)}$ and $P_4^{ss}=1-P_0^{ss}-P_1^{ss}-P_2^{ss}-P_3^{ss}$, where we have used $x_i=k_{\mathrm{on}}c_i/k_{\mathrm{off},i}$. Our generating function transition matrix is

$$\mathbf{M}(\mathrm{s}_1,\mathrm{q}_1,s_2,q_2)=$$
$$\begin{pmatrix}-k_{\mathrm{on}}(c_1+c_2) & k_{\mathrm{off},1} & k_{\mathrm{off},1} & k_{\mathrm{off},2} & k_{\mathrm{off},2}\\ k_{\mathrm{on}}c_1q_1 & -k_{\mathrm{off},1}-\frac{\alpha}{k_{\mathrm{off},1}}+k_p(s_1-1) & 0 & 0 & 0\\ 0 & \frac{\alpha}{k_{\mathrm{off},1}}q_2 & -k_{\mathrm{off},1}+\mathrm{k_p}(s_2-1) & 0 & 0\\ k_{\mathrm{on}}c_2q_1 & 0 & 0 & -k_{\mathrm{off},2}-\frac{\alpha}{k_{\mathrm{off},2}}+k_p(s_1-1) & 0\\ 0 & 0 & 0 & \frac{\alpha}{k_{\mathrm{off},2}}q_2 & -k_{\mathrm{off},2}+k_p(s_2-1)\end{pmatrix}\tag{S5}$$

The generating function approach used above does not lend itself well to this problem. Instead, the mean sensing molecules $\langle\mathbf{n}\rangle=\langle(n_1,m_1,n_2,m_2)\rangle$ can be solved for in steady state by direct solution of the system of ODEs

$$\frac{d\langle\mathbf{n}\rangle}{dt}=\sum_{\mathbf{n}}^{\infty}\sum_i\mathbf{n}\frac{dP_i^{\mathbf{n}}}{dt}.$$

As an example, consider the derivation of $\langle m_1\rangle$. The corresponding ODE to solve is

$$\frac{d\langle m_1\rangle}{dt}=\sum_{m_1}^{\infty}\sum_i m_1\frac{dP_i^{m_1}}{dt}$$

$$=\sum_{m_1=0}^{\infty}m_1\left(k_{on}c_1P_0^{m_1-1}+k_{on}c_2P_0^{m_1-1}-k_{on}(c_1+c_2)P_0^{m_1}\right)$$

$$=\sum_{m_1=0}^{\infty}(m_1+1)k_{on}c_1P_0^{m_1}+(m_1+1)k_{on}c_2P_0^{m_1}-m_1k_{on}(c_1+c_2)P_0^{m_1}$$

$$=\sum_{m_1}^{\infty}k_{on}c_1P_0^{m_1}+k_{on}c_2P_0^{m_1}$$

Terms of the form $\sum_{m_1} P_i^{m_1}$ simplify to the steady state receptor occupancy $P_i$ which we already calculated. Thus, we finally have

$$\frac{d\langle m_1\rangle}{dt} = k_{\text{on}}(c_1 + c_2)P_0^{ss}$$

which is easily integrated to get an expression for $\langle m_1\rangle$.

The resulting mean equations are:

$$\langle n_1\rangle = \frac{k_p t}{(1 + x_1 + x_2)}\left(\frac{x_1}{1 + \alpha/k_{\text{off},1}^2} + \frac{x_2}{1 + \alpha/k_{\text{off},2}^2}\right)$$

$$\langle m_1\rangle = \frac{t}{(1 + x_1 + x_2)}\left(x_1 k_{\text{off},1} + x_2 k_{\text{off},2}\right)$$

$$\langle n_2\rangle = \frac{k_p t\, \alpha}{(1 + x_1 + x_2)}\left(\frac{x_1}{k_{\text{off},1}^2 + \alpha} + \frac{x_2}{k_{\text{off},2}^2 + \alpha}\right)$$

$$\langle m_2\rangle = \frac{t\, \alpha}{(1 + x_1 + x_2)}\left(\frac{x_1 k_{\text{off},1}}{k_{\text{off},1}^2 + \alpha} + \frac{x_2 k_{\text{off},2}}{k_{\text{off},2}^2 + \alpha}\right)$$

The covariance matrix of the sensing molecules is harder to solve because the corresponding ODEs for the sensing molecules $\mathbf{n}$, i.e.

$$\frac{d\langle n_k^2\rangle}{dt} = \sum_{\mathbf{n}}^{\infty}\sum_i n_k^2 \frac{dP_i^{\mathbf{n}}}{dt} \tag{S6}$$

have terms of the form

$$\langle n_k\rangle_i = \sum_{\mathbf{n}}^{\infty} n_k P_i^{\mathbf{n}}\,.$$

We can obtain analytic expressions for these terms by solving the related system of ODEs

$$\frac{d\langle n_k\rangle_i}{dt} = \sum_{\mathbf{n}}^{\infty} n_k \frac{dP_i^{\text{n}}}{dt}$$

This is a non-homogenous system of ODEs which can be solved by variation of parameters. Applying this technique for each sensing molecule $n_k$, we can then replace the $\langle n_k\rangle_i$ terms in Eq. (S6) with functions that are independent of $n_k$ and thereby obtain a separable system of equations which can be integrated to give mean square data. The covariance matrix follows immediately from this procedure, but the results are too cumbersome to present here in closed form. For additional computational details we refer the reader to the Mathematica notebook provided at the beginning of the Supplementary Material.

## Section B: Obtaining Maximum Likelihood Estimates of $c$ and $k_{\text{off}}$

To generalize the notation across our models we denote the $d$-dimensional vector of observables by $\mathbf{n}$ and the model parameters (which could be $c$, $k_{\text{off}}$, or both) by $\boldsymbol{\theta}$. We consider the estimates one could make for $\boldsymbol{\theta}$ based on the probability of having observed the data $\mathbf{n}$ given unknown true values of the model parameters, known as the likelihood, $P(\mathbf{n}|\boldsymbol{\theta})$.

Model inference generally involves maximizing a related quantity, the posterior for $\boldsymbol{\theta}$ given $\mathbf{n}$, $P(\boldsymbol{\theta}|\mathbf{n}) = \frac{P(\mathbf{n}|\boldsymbol{\theta})P(\boldsymbol{\theta})}{P(\mathbf{n})}$, where $P(\boldsymbol{\theta})$ is often called the prior [72]. When $P(\boldsymbol{\theta})$ is uniform, maximizing the posterior is equivalent to maximizing the likelihood. For simplicity we consider this case here; constraints on $\boldsymbol{\theta}$ can be incorporated via a non-uniform prior [72].

$P(\mathbf{n}|\boldsymbol{\theta})$ is determined by the stochastic dynamics of the receptor signalling process. We find that in the long time limit, $\min(k_{\mathrm{off}}, k_p) \gg 1/t$, the likelihood is well approximated by a Gaussian (see Section E),

$$P(\mathbf{n}|\boldsymbol{\theta}) = \frac{1}{\sqrt{(2\pi)^d |\mathbf{C}(\boldsymbol{\theta})|}} \exp\left(-\frac{1}{2}\left(\mathbf{n} - \boldsymbol{\mu}(\boldsymbol{\theta})\right)^{\mathrm{T}} \mathbf{C}(\boldsymbol{\theta})^{-1}\left(\mathbf{n} - \boldsymbol{\mu}(\boldsymbol{\theta})\right)\right) \quad \text{(S7)}$$

where $\boldsymbol{\mu}(\boldsymbol{\theta})$ is the vector of data means, and $\mathbf{C}(\boldsymbol{\theta})$ is the data covariance matrix found from the generating function approach for a given ligand-receptor signalling scheme. The functional forms of $\boldsymbol{\mu}(\boldsymbol{\theta})$, $\mathbf{C}(\boldsymbol{\theta})$ are provided in Section A for the various models we consider.

A maximum likelihood estimate (MLE) $\boldsymbol{\theta}^*$ can be found by solving $\boldsymbol{\nabla}_{\boldsymbol{\theta}} \mathrm{L}\big|_{\boldsymbol{\theta}^*} = \mathbf{0}$ where $L = \ln P$. This is generally only possible to do numerically. However, if we neglect the $\ln(1/\sqrt{(2\pi)^d |\mathbf{C}|})$ term in $L$, the MLE can be found immediately as the inverse function of the means $\boldsymbol{\theta}_{\mathrm{est}}(\mathbf{n}) \equiv \boldsymbol{\mu}(\boldsymbol{\theta})^{-1}$. This "heuristic MLE" $\boldsymbol{\theta}_{\mathrm{est}}(\mathbf{n})$ is readily found for each of the models we consider. We find excellent agreement between this heuristic MLE and the full numeric MLE of the Gaussian likelihood (see Figures S1 and S2).

An estimator is said to be unbiased when $\mathrm{E}[\boldsymbol{\theta}_{\mathrm{est}}(\mathbf{n})] = \boldsymbol{\theta}$. We note that our inverse-mean estimator is essentially unbiased when the likelihood is sharply peaked around the mean [72], as it is in the long time limit which we focus on.

## *MLE for Model 1*

The likelihood of observing $n$ molecules of the product in Model 1 is

$$P(n|c, k_{\mathrm{off}}) \approx \frac{1}{\sqrt{2\pi\langle\delta n^2\rangle}} e^{\frac{-(n-\langle n\rangle)^2}{2\langle\delta n^2\rangle}}. \quad \text{(S8)}$$

The full MLE estimate is determined by the condition

$$\frac{(n - \langle n\rangle)}{2\langle\delta n^2\rangle}\frac{\partial\langle n\rangle}{\partial x} - \frac{1}{2}(n - \langle n\rangle)^2 \frac{\partial}{\partial x}\left(\frac{1}{\langle\delta n^2\rangle}\right) - \frac{1}{2}\frac{\partial}{\partial x}\ln\langle\delta n^2\rangle = 0$$

Neglecting the logarithmic term produces the heuristic MLE estimate described above,

$$n = \langle n\rangle(x^*) \;\Rightarrow\; x^* = \frac{n}{k_p t - n} \quad \text{(S9)}$$

which agrees well with the full numerical MLE up until $n \approx k_p t$ (see Fig. S1). Recall that $\langle n\rangle = k_p t P_1^{ss} = k_p t \frac{x}{(1+x)}$, so that $n > k_p t$ is more likely to occur when the receptor is saturated. In this scenario our heuristic estimate breaks down entirely. This can be resolved by either a non-uniform prior or by heuristically estimating $x \to \infty$ when $n > k_p t$. This breakdown is not completely unrealistic, as a cell's sensing ability may be expected to be inaccurate when the receptor is saturated.

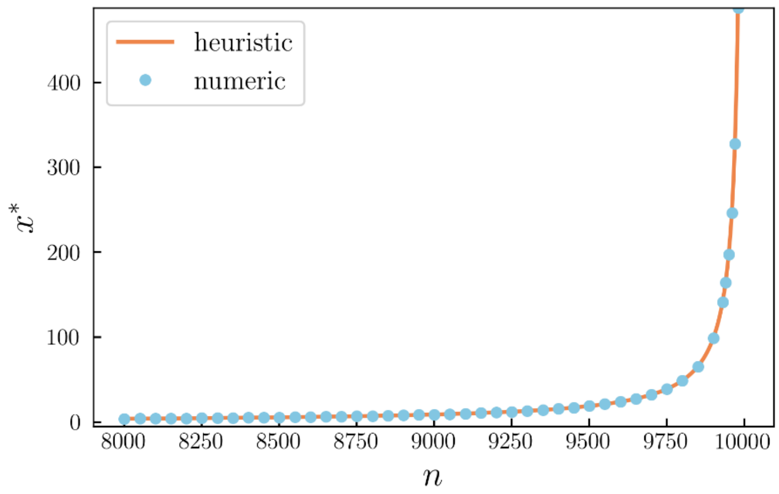


FIG. S1. The MLE for $x$ as a function of $n$. The orange line is the heuristic MLE (Eq. (S9)) while the blue dots are the true peak of the likelihood (Eq. (S8)), found numerically. Parameters: $k_p t = 10^4$, $k_{\text{off}}/k_{\text{on}} = 10^{-7}$. The value of $c$ was estimated and converted to $x^*$ using known $K_D = k_{\text{off}}/k_{\text{on}}$.

## *MLE for Model 2*

The likelihood is given by

$$P(n,m|c,k_{\text{off}}) = \frac{1}{\sqrt{(2\pi)^2|\mathbf{C}|}} \exp\left\{-\frac{1}{2}\begin{pmatrix} n-\langle n\rangle \\ m-\langle m\rangle \end{pmatrix}^{\mathrm{T}} \mathbf{C}^{-1}\begin{pmatrix} n-\langle n\rangle \\ m-\langle m\rangle \end{pmatrix}\right\} \tag{S10}$$

$$\text{where } \mathbf{C} = \begin{pmatrix} \langle \delta n^2\rangle & \langle \delta n \delta m\rangle \\ \langle \delta n \delta m\rangle & \langle \delta m^2\rangle \end{pmatrix}.$$

Once again, we find that the heuristic MLE (Eq. (9) in main text) agrees well with the numeric MLE for small $c$ and $k_{\text{off}}$ (Fig. S2).

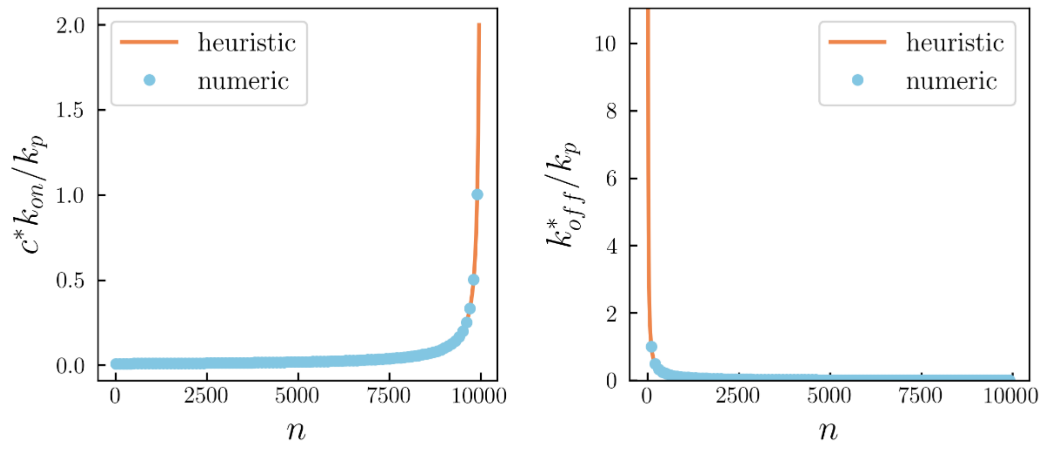

FIG. S2. Model 2 MLE as a function of n for fixed m. The cell can estimate $c$ and $k_{\text{off}}$ separately. The orange lines correspond to the heuristic estimators for $c^*$ and $k_{\text{off}}{}^*$ while the blue dots show the true peak of the distribution as found numerically. Parameters are $k_p t = 10^4, k_p/k_{on} = 10$, m $= 100$.

## *MLE for Model 3*

A peculiarity of the model used in the main text is that when $k_f$ is treated as a constant, the four variables $n_1, n_2, m_1, m_2$ are not independent and thus do not contain enough information to determine both the dissociation rates and the concentrations of both ligands. Mathematically, the Jacobian of the data means with respect to the ligand parameters (i.e. $\partial\mu_i/\partial\theta_j$) is everywhere singular, so that heuristic MLEs cannot be obtained. This problem disappears in a more general case where $k_f$ is a function of the ligand identity. The physical reasoning behind this choice is that the transition rates between different bound states is partially determined by the identity of the ligand, much like the $k_{\text{off}}$. We choose $k_f \propto 1/k_{\text{off}}$ based on the intuitive notion that strong binding ligands should move to the second proofreading state faster than weak binding ligands. The results do not depend on this specific assumption, and other functional forms of $k_f$ are viable, as long as the $n_1, n_2, m_1, m_2$ variables are functionally independent.

Repeating the same process for the multi-state scheme (Model 3) using the means and variances for the $n$'s and $m$'s derived in Section A, we obtain heuristic estimators for $c_1$, $k_{\text{off},1}$, $c_2$ and $k_{\text{off},2}$:

$$c_1^* = \frac{k_p m_1 + \frac{\gamma_1}{\gamma_2}\sqrt{\alpha\gamma_2}}{2k_{\text{on}}\left(k_p t - (n_1 + n_2)\right)}$$

$$c_2^* = \frac{k_p m_1 - \frac{\gamma_1}{\gamma_2}\sqrt{\alpha\gamma_2}}{2k_{\text{on}}\left(k_p t - (n_1 + n_2)\right)}$$

$$k_{\text{off},1}^* = \frac{k_p\alpha(m_2 n_1 - m_1 n_2 + m_2 n_2) - \sqrt{\alpha\gamma_2}}{2\left(k_p^2 m_2^2 - n_1 n_2 \alpha\right)}$$

$$k_{\text{off},2}^* = \frac{k_p\alpha(m_2 n_1 - m_1 n_2 + m_2 n_2) + \sqrt{\alpha\gamma_2}}{2\left(k_p^2 m_2^2 - n_1 n_2 \alpha\right)}$$

where,

$$\gamma_1 = k_p^2(m_1^2 n_2 + (n_1 + n_2)(2m_2^2 - 3m_1 m_2)) + 2n_1^2\alpha(n_1 + n_2)$$

$$\gamma_2 = 4k_p^4 m_2^3(m_1 - m_2) + k_p^2\alpha((m_1 - m_2)^2 n_2^2 - 6m_2(m_1 - m_2)n_1 n_2 - 3m_2^2 n_1^2) + 4n_1^3 n_2 \alpha^2.$$

As our focus in this paper is on the specificity and accuracy bounds for these MLEs we will not comment further on these results.

# Section C: Accuracy of the estimators

## *Full expression for the Fisher Information Matrix*

### *Non-pleiotropic receptor*

For a simple one-variable non-pleiotropic receptor, the log-likelihood is

$L(c;n) = -\frac{1}{2v(c)}\left(n - \langle n\rangle(c)\right)^2 - \frac{1}{2}\ln\left(2\pi v(c)\right)$

where $v(c) = \langle \delta n^2 \rangle$. Thus

$$-\frac{\partial^2 L}{\partial c^2} = \frac{1}{v}\left(\frac{\partial\langle n\rangle}{\partial c}\right)^2 - \frac{\partial}{\partial c}\left(\frac{1}{v}\frac{\partial\langle n\rangle}{\partial c}\right)(n - \langle n\rangle) - \frac{1}{2}\frac{\partial}{\partial c}\left(\frac{1}{v^2}\frac{\partial v}{\partial c}\right)(n - \langle n\rangle)^2 + \frac{1}{2}\frac{1}{v^2}\frac{\partial v}{\partial c}\frac{\partial\langle n\rangle}{\partial c}(n - \langle n\rangle) + \frac{1}{2}\frac{\partial^2}{\partial c^2}\ln(v)$$

Averaging over $n$ gives for the Fisher Information

$$\boldsymbol{\mathcal{I}} = \langle -\frac{\partial^2 L}{\partial c^2}\rangle = \frac{1}{v}\left(\frac{\partial\langle n\rangle}{\partial c}\right)^2 - \frac{1}{2}\frac{\partial}{\partial c}\left(\frac{1}{v^2}\frac{\partial v}{\partial c}\right)v + \frac{1}{2}\frac{\partial^2}{\partial c^2}\ln(v) = \frac{1}{v}\left(\frac{\partial\langle n\rangle}{\partial c}\right)^2 + \frac{1}{2}\left(\frac{1}{v}\frac{\partial v}{\partial c}\right)^2$$

In the long time limit, the first term in this expression scales like $\sim t$, and asymptotically dominates the second term which scales as a constant.

## *General formalism*

We are interested in the error of our estimate for $\boldsymbol{\theta}$ (i.e. $c, k_{\text{off}}$), which is related to the width of the posterior $P(\boldsymbol{\theta}|\mathbf{n}) = \frac{P(\mathbf{n}|\boldsymbol{\theta})P(\boldsymbol{\theta})}{P(\mathbf{n})}$ about its peak [72]. To obtain an estimate of the error, we approximate the Cramer-Rao lower bound on the error and check the quality of that approximation. The prior, $P(\boldsymbol{\theta})$, is assumed to be uniform here, so maximizing the posterior is equivalent to maximizing the likelihood as in Section B [72].

Likelihood functions are often difficult to extremize analytically; various approaches might therefore be considered to obtain estimates $\widehat{\boldsymbol{\theta}}$ of the model parameters (e.g. the vector of estimates $\widehat{\boldsymbol{\theta}} = \begin{bmatrix}\hat{c}\\ \hat{k}_{\text{off}}\end{bmatrix}$ for our ligand sensing problem). Each approach has an associated covariance matrix $\boldsymbol{\Sigma}_{\widehat{\boldsymbol{\theta}}}$ describing the typical deviation with respect to the true value $\boldsymbol{\theta}$. The most accurate estimator one could construct from a likelihood function is constrained by the Fisher information matrix (FIM) [72], defined as

$$\mathcal{I}(\boldsymbol{\theta})_{ij} = \mathrm{E}\left[\frac{\partial L}{\partial\theta_i}\frac{\partial L}{\partial\theta_j}\right] = \int P(\mathbf{n}|\boldsymbol{\theta})\frac{\partial L}{\partial\theta_i}\frac{\partial L}{\partial\theta_j}\, d\mathbf{n} \tag{S11}$$

where $L = P(\mathbf{n}|\boldsymbol{\theta})$. The Cramer-Rao lower bound (CRLB) states the following limit on the accuracy of an unbiased estimator $\widehat{\boldsymbol{\theta}}$: $\boldsymbol{\Sigma}_{\widehat{\boldsymbol{\theta}}} \geq \boldsymbol{\mathcal{I}}^{-1}$ [72]. Under certain regularity conditions on $L$ [72], Eq. (S11) has an alternative form - the negative Hessian of $L$, $\mathcal{I}(\boldsymbol{\theta})_{ij} = \mathrm{E}\left[-\frac{\partial^2 L}{\partial\theta_i\partial\theta_j}\right]$, which coincides with the intuitive explanation for the estimation error shown in the main text. For Normally distributed data $\mathbf{n} \sim \mathcal{N}\left(\boldsymbol{\mu}(\boldsymbol{\theta}), \hat{\mathbf{C}}(\boldsymbol{\theta})\right)$ to which the distributions converge at long times in our case (see Eq. (S10) and Section E), $\boldsymbol{\mathcal{I}}(\boldsymbol{\theta})$ has an exact form [72]

$$\mathcal{I}(\boldsymbol{\theta})_{ij} = \frac{\partial\boldsymbol{\mu}^{\mathrm{T}}}{\partial\theta_i}\hat{\mathbf{C}}^{-1}\frac{\partial\boldsymbol{\mu}}{\partial\theta_j} + \frac{1}{2}\mathrm{tr}\left(\hat{\mathbf{C}}^{-1}\frac{\partial\hat{\mathbf{C}}}{\partial\theta_i}\hat{\mathbf{C}}^{-1}\frac{\partial\hat{\mathbf{C}}}{\partial\theta_j}\right) \tag{S12}$$

At large $t$, the first term dominates and is used to derive the analytical expressions in the main text.

This dominant term in Eq. (S12) can also be understood through a heuristic derivation using the approximate MLE estimator $\boldsymbol{\theta}_{\text{est}}(\mathbf{n}) = \boldsymbol{\mu}^{-1}(\mathbf{n})$ (Section B). Fluctuations of values of $\mathbf{n}$ around $\boldsymbol{\mu}(\boldsymbol{\theta})$ cause

deviations from the true value, $\delta\boldsymbol{\theta}_{\text{est}} = \boldsymbol{\theta}_{\text{est}}(\mathbf{n}) - \boldsymbol{\theta}$. Since $\boldsymbol{\theta}_{\text{est}}(\boldsymbol{\mu}) = \boldsymbol{\theta}$ by definition, Taylor expanding about the mean gives $\delta\boldsymbol{\theta}_{\text{est}} \approx \frac{\partial\boldsymbol{\theta}_{\text{est}}}{\partial\mathbf{n}}|_{\mathbf{n}=\boldsymbol{\mu}}\delta\mathbf{n}$, where $\frac{\partial\boldsymbol{\theta}_{\text{est}}}{\partial\mathbf{n}} \equiv \hat{\mathbf{J}}$ denotes the Jacobian with the elements $\frac{\partial(\theta_{\text{est}})_i}{\partial \mathrm{n}_j}$. Thus, the covariance matrix of $\delta\boldsymbol{\theta}_{\text{est}}$ is

$$\boldsymbol{\Sigma}_{\text{est}} = \langle \delta\boldsymbol{\theta}_{\text{est}}\delta\boldsymbol{\theta}_{\text{est}}^{\mathrm{T}}\rangle_{P(\mathbf{n}|\boldsymbol{\theta})} = \langle \left(\frac{\partial\boldsymbol{\theta}_{\text{est}}}{\partial\mathbf{n}}|_{\mathbf{n}=\boldsymbol{\mu}}\delta\mathbf{n}\right)\left(\frac{\partial\boldsymbol{\theta}_{\text{est}}}{\partial\mathbf{n}}|_{\mathbf{n}=\boldsymbol{\mu}}\delta\mathbf{n}\right)^{\mathrm{T}} \rangle \approx \hat{\mathbf{J}}(\boldsymbol{\theta})\,\mathbf{C}\,\hat{\mathbf{J}}(\boldsymbol{\theta})^{\mathrm{T}} \quad \text{(S13)}$$

where the averaging over the distribution of $\mathbf{n}$, $\hat{\mathbf{J}}(\boldsymbol{\theta}) = \frac{\partial\boldsymbol{\theta}_{\text{est}}}{\partial\mathbf{n}}|_{\mathbf{n}=\boldsymbol{\mu}(\boldsymbol{\theta})}$, and we have used the fact that $\langle \delta\mathbf{n}\,\delta\mathbf{n}^{\mathrm{T}}\rangle = \hat{\mathbf{C}}$. Since $\boldsymbol{\theta}_{\text{est}}(\boldsymbol{\mu}(\boldsymbol{\theta})) = \boldsymbol{\theta}$, the inverse function theorem gives

$$\boldsymbol{\Sigma}_{\text{est}} = \left(\frac{\partial\boldsymbol{\mu}^{\mathrm{T}}}{\partial\boldsymbol{\theta}}\hat{\mathbf{C}}^{-1}\frac{\partial\boldsymbol{\mu}}{\partial\boldsymbol{\theta}}\right)^{-1} \quad \text{(S14)}$$

We used the heuristic Eq. (S14) to obtain the analytical expressions for the estimate covariance matrix for each of our models in the main text for Models 1, 2.

## *Estimation Error for Model 2*

The elements of the estimate covariance matrix in the long time limit are

$$\begin{aligned} \langle \delta c^2 \rangle &= \frac{\mathrm{c}^2}{\mathrm{k_p}t}\frac{(1+x)}{\mathrm{x}}\left(x^2 + \frac{\mathrm{k_p}}{k_{\text{off}}}\right) \\ \langle \delta k_{\text{off}}^2 \rangle &= \frac{k_{\text{off}}^2}{\mathrm{k_p}t}\frac{(1+x)}{\mathrm{x}}\left(1 + \frac{\mathrm{k_p}}{k_{\text{off}}}\right) \\ \langle \delta c \delta k_{\text{off}} \rangle &= \frac{c k_{\text{off}}}{k_p t}(1+x) \end{aligned} \quad \text{(S15)}$$

## *Estimation Error for Model 3*

The elements of the estimate covariance matrix are obtained in the same method as outlined above once the data covariance matrix has been obtained (see Section A), but the results are far too cumbersome to present in closed form. This motivates our numerical analysis of the crosstalk sensing performance presented in the main text.

## *Comparison of Heuristic Covariance to the full CRLB*

To compare the $\boldsymbol{\Sigma}^A \equiv \boldsymbol{\Sigma}_{\text{est}}$ (heuristic) and $\boldsymbol{\Sigma}^B \equiv \hat{\boldsymbol{\mathcal{I}}}^{-1}$ (exact) errors of the estimates we computed the ratio of their determinants, $\frac{\det(\boldsymbol{\Sigma}^A)}{\det(\boldsymbol{\Sigma}^B)}$. The quantity $\det(\boldsymbol{\Sigma})$ serves as a measure of the estimate error and can be understood as a measure of the combined error in joint estimation of $c$ and $k_{\text{off}}$ [50].

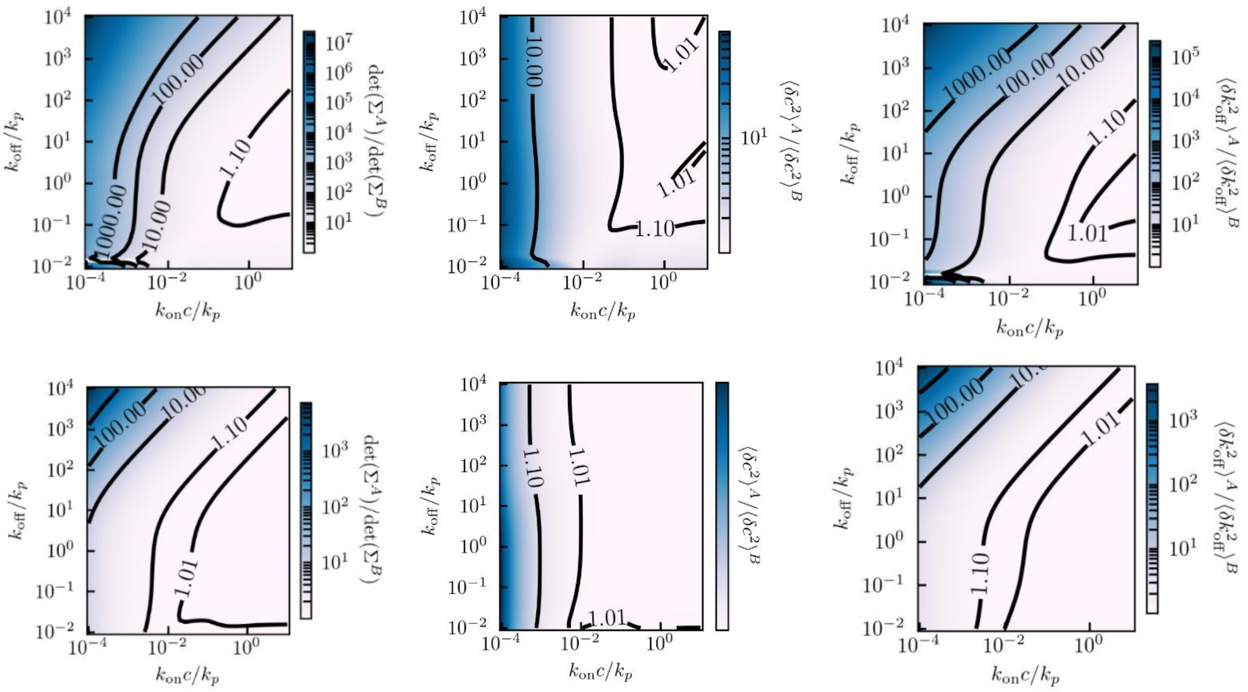


FIG. S3. Comparison of heuristic estimation error and the Cramer-Rao lower bound for Model 2. Top Panels: Comparison of heuristic estimates of the determinants and diagonal terms of $\mathbf{\Sigma}^A$ to the determinant and diagonal terms of $\mathbf{\Sigma}^B$ (the full CRLB) for Model 2 for $k_p t = 10^2$. Bottom Panels: Corresponding plots for $k_p t = 10^4$. The contour line of 1.10 corresponds to a ratio below which the determinants and diagonal terms of $\mathbf{\Sigma}^A$ is within ten percent of the corresponding values of $\mathbf{\Sigma}^B$.

We generally find that the heuristic estimate $\boldsymbol{\theta}_{\rm est}(\mathbf{n})$ performs well in the regime of interest (Fig. S3) as $k_p t$ increases, and fails to approach the full CRLB, $\mathbf{\Sigma}^B$, when $x \ll 1$, in which regime the estimate accuracy is already low due to insufficient number of binding events. We also demonstrated that the error in the heuristic estimates obtained by Eq. (S14) approach the full CRLB for a wide range of parameter values tested. In regions where the error ratio is large, the error in the estimate can be improved by considering information in how the data covariance depends on the parameters.

# Section D: Alternative calculation of the moments of the distribution of $n$ and $m$

## *Moments of the distribution of $n$*

The master equation describing the process is

$$P_1(t) = k_{\rm on} P_0(t) - k_{\rm off} P_1(t) \tag{S16}$$

$$P_0(t) = -k_{\rm on} P_0(t) + k_{\rm off} P_1(t)$$

Where $P_1(t)$ is the probability to be in the state “1” at time $t$. Of course, $P_1(t) + P_0(t) = 1$ at any $t$. The steady state solution to this equation is $\left(P_0(t), P_1(t)\right) = \left(\frac{k_{\rm off}}{k_{\rm off}+k_{\rm on}}, \frac{k_{\rm on}}{k_{\rm off}+k_{\rm on}}\right) \equiv \vec{P}^{ss}$

Let us introduce a random variable $\hat{h}(t)$ whose value is 1 when the system is in state "1", and zero if system is in state "0". Then the total bound time for a given trajectory of bound-unbound times is $\hat{t}_b = \int_0^t \hat{h}(t')dt'$.

The average bound time is

$$\langle t_b \rangle = \int_0^t \langle \hat{h}(t') \rangle dt' = \int_0^t [1 \cdot P_1(t') + 0 \cdot P_0(t')]dt' \tag{S17}$$

Now, the time dependent solution of Eq. (S16) is $P_1(t) = P_1^{ss}(1 - e^{-rt}) + P_1(0)e^{-rt}$, where $r = k_{\text{on}} + k_{\text{off}}$ and $P_1(0)$ is the probability to be in state 1 at time $t = 0$. Assuming that the system starts at the steady state, $P_1(0) = P_1^{ss}$, Eq. (S17) gives $\langle t_b \rangle = P_1^{ss} t$, as expected intuitively: $P_1^{ss}$ is the fraction of time the system spends in state 1.

To calculate the variance of $\hat{t}_b$, let us first calculate its second moment:

$$\langle t_b^2 \rangle = \int_0^t dt'' \int_0^t dt' \, \langle \hat{h}(t') \, \hat{h}\,(t'') \rangle = \int_0^t dt'' \int_0^{t''} dt' \, \langle \hat{h}(t') \, \hat{h}\,(t'') \rangle + \int_0^t dt'' \int_{t''}^t dt' \, \langle \hat{h}(t') \, \hat{h}\,(t'') \rangle$$

$$= \int_0^t dt'' \int_0^{t''} dt' \, \langle \hat{h}(t') \, \hat{h}\,(t'') \rangle + \int_0^t dt' \int_0^{t'} dt'' \, \langle \hat{h}(t') \, \hat{h}\,(t'') \rangle$$

$$= 2 \int_0^t dt'' \int_0^{t''} dt' \, \langle \hat{h}(t') \, \hat{h}\,(t'') \rangle \tag{S18}$$

Now, for $t'' > t'$,

$$\langle \hat{h}(t') \, \hat{h}\,(t'') \rangle = P(h = 1, t''; h = 1, t') = P(h = 1, t'' | h = 1, t') P_1^{ss} = P_1(t'' | P_1(t') = 1) P_1^{ss}$$

Thus,

$$\langle \hat{h}(t') \, \hat{h}\,(t'') \rangle = \left[ P_1^{ss} \left(1 - e^{-r(t''-t')}\right) + 1 \cdot e^{-r(t''-t')} \right] P_1^{ss} = P_1^{ss} [e^{-r(t''-t')}(1 - P_1^{ss}) + P_1^{ss}]$$

Therefore,

$$2 \int_0^t dt'' \int_0^{t''} dt' \, \langle \hat{h}(t') \, \hat{h}\,(t'') \rangle = 2P_1^{ss} \int_0^t dt'' \int_0^{t''} dt' \left[ e^{-r(t''-t')}(1 - P_1^{ss}) + P_1^{ss} \right]$$

$$= (P_1^{ss})^2 t^2 + 2P_1^{ss}(1 - P_1^{ss}) \left[ \frac{t}{r} - \frac{1}{r^2}(1 - e^{-rt}) \right]$$

Finally, the variance is

$$\langle t_b^2 \rangle - \langle t_b \rangle^2 = 2P_1^{ss}(1 - P_1^{ss}) \left[ \frac{t}{r} - \frac{1}{r^2}(1 - e^{-rt}) \right]$$

$$= \frac{t}{k_{\text{off}}} \frac{2x}{(1+x)^3} \left[ 1 - \frac{1}{k_{\text{off}} t(1+x)} \left(1 - e^{-k_{\text{off}} t(1+x)}\right) \right] \tag{S19}$$

where $x = \frac{k_{\text{on}}}{k_{\text{off}}}$.

In the limit $k_{\text{off}} t \gg 1$, $\langle t_b^2 \rangle - \langle t_b \rangle^2 \simeq \frac{k_{\text{off}} t}{k_{\text{off}}^2} \frac{2x}{(1+x)^3}$.

In the $t \to 0$ limit, the leading term is $\langle t_b^2 \rangle - \langle t_b \rangle^2 \simeq \frac{(k_{\text{off}} t)^2}{k_{\text{off}}^2} \frac{x}{(1+x)^2} = t^2 \frac{x}{(1+x)^2}$.

The moments of the distribution of $n$ can be calculated as follows. For a given value of $t_b$, the probability distribution of $n$, $P(n|t_b)$ is a Poisson distribution with the mean and the variance $k_p t_b$. Therefore

$$\langle n\rangle = \sum_n nP(n) = \sum_n n \int dt_b \langle t_b^2\rangle - \langle t_b\rangle^2 P(n|t_b)P(t_b)$$

$$= \int dt_b k_p t_b P(t_b) = k_p\langle t_b\rangle = k_p t \frac{x}{1+x}$$

in agreement with the expression in the main text. Similarly

$$\langle n^2\rangle = \sum_n n^2 P(n) = \sum_n n^2 \int dt_b P(n|t_b)P(t_b)$$

$$= \int dt_b \left(k_p t_b + \left(k_p t_b\right)^2\right) P(t_b) \ = k_p\langle t_b\rangle + k_p^2\langle t_b^2\rangle$$

$$= k_p\langle t_b\rangle + k_p^2\langle t_b\rangle^2 + k_p^2\left(\langle t_b^2\rangle - \langle t_b\rangle^2\right).$$

Thus

$$\langle n^2\rangle - \langle n\rangle^2 = k_p\langle t_b\rangle + k_p^2\left(\langle t_b^2\rangle - \langle t_b\rangle^2\right) = \frac{k_p t x}{1+x} + \frac{2k_p^2 t}{k_{\text{off}}}\frac{x}{(1+x)^3}$$

in accord with the expression in the main text.

## *Moments of the distribution of m*

The moments of $m$ can be calculated using renewal theory [94]. To this end, we notice that the time series of the receptor occupancy can be viewed as the sequence of identically distributed binding-unbinding cycles.

The probability density that one binding-unbinding cycle takes time $t$ is the convolution of the binding and unbinding time distributions

$$Q(t) = \int_0^t dt' k_{\text{off}} e^{-k_{\text{off}}(t-t')} k_{\text{on}} e^{-k_{\text{on}}t'} = \frac{k_{\text{on}}c\, k_{\text{off}}}{k_{\text{on}}c - k_{\text{off}}}\left(e^{-k_{\text{off}}t} - e^{k_{\text{on}}c\, t}\right) \qquad (S20)$$

The average time of each such cycle is

$$\bar{t}_1 = \int dt\, t\, Q(t) = \frac{k_{\text{on}}c + k_{\text{off}}}{k_{\text{on}}c\, k_{\text{off}}} \equiv \frac{1}{r_{\text{eff}}} \qquad (S21)$$

and the variance is

$$\sigma_1^2 = \int dt\, t^2 Q(t) - \bar{t}_1^2 = \frac{(k_{\text{on}}c)^2 + k_{\text{off}}^2}{(k_{\text{on}}c)^2 k_{\text{off}}^2} \qquad (S22)$$

It can be shown [94] that in the limit $k_{\text{off}}t \gg 1$, the probability distribution of the number of binding-unbinding cycles $m$ converges to a normal distribution with the mean

$$\langle m\rangle = t/\bar{t}_1 \ = k_{\text{off}} t \frac{x}{1+x}$$

and the variance

$$\mathrm{var}(m) = \frac{t\,\sigma_1^2}{\bar{t}_1^3} = k_{\mathrm{off}} t \frac{x(1+x^2)}{(1+x)^3}$$

in agreement with the expressions in the main text obtained from the full master equation.

# Section E: Long time distribution well-approximated by a Normal distribution

In this section, we show that in the long time limit the distributions of $n$ and $m$ are well approximated by a Normal distribution. The long time limit we consider is defined by $\min(k_{\mathrm{off}}, k_p) \gg 1/t$. When this is satisfied, the sensing variable distributions from the master equation solution tend to a normal distribution. One needs $k_{\mathrm{off}} t \gg 1$ to produce sufficiently many binding-unbinding events, and $k_p t \gg 1$ to ensure sufficient production of $n$.

To understand why the distributions limit to Gaussians, first note that the receptor bound time $\tau_b \sim \mathrm{Exp}(k_{\mathrm{off}})$ and unbound time $\tau_u \sim \mathrm{Exp}(k_{\mathrm{on}} c)$. Both $n$ and $m$ are constructed from the distribution of bound/unbound times.

The time between binding events (which produce $m$) are independent and identically distributed (iid) random variables, $\tau = \tau_b + \tau_u$. The sum of two exponentials is a hypoexponential distribution, with mean $\langle \tau \rangle = \frac{1}{k_{\mathrm{on}} c} + \frac{1}{k_{\mathrm{off}}}$ and variance $\sigma^2 = \frac{1}{(k_{\mathrm{on}} c)^2} + \frac{1}{k_{\mathrm{off}}^2}$. In renewal theory, one denotes the sequence of $\tau_i$ as interarrival times, and $m(t)$ as the associated counting process. By the central limit theorem for counting processes [94], we have $\lim_{t\to\infty} m(t) \sim N(\mu, V)$ with $\mu = \langle \tau \rangle^{-1} t, V = \sigma^2 \langle \tau \rangle^{-3} t$ (in agreement with Eq. (7)).

The phosphorylation readout $n$, which is a sum of Poisson distributed production events accruing during each bound time $\tau_b$, also adheres to CLT. We may write $n = \sum_{i=1}^m X_i$, where $X_i$ is Poisson distributed with parameter $\lambda_i = k_p \tau_b^{(i)}$. One way to see that $n$ is Gaussian at long times is through the Lyapunov criterion [95]. Define $\mu_i \equiv \mathrm{E}[X_i]$ and $s_m^2 \equiv \sum_{i=1}^m \mathrm{Var}(X_i)$. The Lyapunov criterion states that $\frac{1}{s_m} \sum_{i=1}^m (X_i - \mu_i)$ converges to a unit Gaussian provided that $\lim_{m\to\infty} \frac{1}{s_m^{2+\delta}} \sum_{i=1}^m \mathrm{E}\big[|X_i - \mu_i|^{2+\delta}\big] = 0$ for some $\delta > 0$.

When $\delta = 2$, it is easy to see that the criterion holds in our case, where we have $\mu_i = \lambda_i$ and $s_m^2 = \sum_{i=1}^m \lambda_{\mathrm{i}}$. Also note the fourth central moment of $X_i \sim \mathrm{Pois}(\lambda_{\mathrm{i}})$ is $\mu_4 = \lambda_i(1 + 3\lambda_i)$. Then the condition simplifies as

$$\lim_{m\to\infty} \frac{\sum_{i=1}^m \lambda_i (1+3\lambda_i)}{\left(\sum_{i=1}^m \lambda_{\mathrm{i}}\right)^2} = \lim_{m\to\infty} 3 \frac{\sum_{i=1}^m \lambda_i^2}{\left(\sum_{i=1}^m \lambda_{\mathrm{i}}\right)^2} = \lim_{m\to\infty} 3 \frac{1}{1 + \frac{\sum_{i=1}^m \lambda_i \sum_{j\neq i}^m \lambda_j}{\sum_{i=1}^m \lambda_i^2}}.$$

For the Lyapunov criterion to hold, we therefore need that $\sum_{i=1}^m \lambda_i \sum_{j\neq i}^m \lambda_j > \sum_{i=1}^m \lambda_i^2$ asymptotically. Note that as $m$ gets large, the sums can be approximated as $\lim_{m\to\infty} \sum_{j\neq i}^m \lambda_j \approx \lim_{m\to\infty} (m-1)\langle \lambda \rangle = \lim_{m\to\infty} (m-1) k_{\mathrm{p}} \langle t_b \rangle$ and $\lim_{m\to\infty} \sum_{i=1}^m \lambda_i^2 \approx \lim_{m\to\infty} m \langle \lambda^2 \rangle = \lim_{m\to\infty} m k_{\mathrm{p}}^2 \langle t_b^2 \rangle$. Therefore,

$$3 \lim_{m\to\infty} \frac{1}{1 + \frac{\sum_{i=1}^m \lambda_i \sum_{j\neq i}^m \lambda_j}{\sum_{i=1}^m \lambda_i^2}} \approx \lim_{m\to\infty} \frac{1}{1 + \frac{\sum_{i=1}^m \lambda_i (m-1) k_{\mathrm{p}} \langle t_b \rangle}{m k_{\mathrm{p}}^2 \langle t_b^2 \rangle}} = \lim_{m\to\infty} \frac{1}{1 + \frac{m(m-1)\langle t_b \rangle^2}{m \langle t_b^2 \rangle}}.$$

Using previous definitions of $\langle t_b \rangle$ and $\langle t_b^2 \rangle$ for $k_{\text{off}}t \gg 1$ derived in Section D, we may write

$$\lim_{m\to\infty} \frac{1}{1+(m-1)\dfrac{\dfrac{x^2}{(1+x)^2}t^2}{\dfrac{x^2}{(1+x)^2}t^2+\dfrac{2tx}{k_{\text{off}}(1+x)^2}}} = \lim_{m\to\infty} \frac{1}{1+(m-1)\dfrac{1}{1+\dfrac{2}{k_{\text{off}}tx}}} = 0.$$

Thus, according to the Lyapunov criterion, we find that $n$ is Gaussian at long times ($m \to \infty$).

To numerically demonstrate the long time distributions, we use the Gillespie algorithm to simulate the dynamics described by our master equations. Fig. S4 shows representative comparisons between the simulations and Normal distributions for Model 2 with moments derived from the generating functions of the master equation. Similar Normal distributions are obtained for Models 1 and 3. Simulations performed for the following dimensionless parameters: $\frac{k_{\text{on}}c}{k_p} = \frac{1}{80}, \frac{k_{\text{off}}}{k_p} = \frac{50}{80},\ k_p t = 3680, g = 5.$

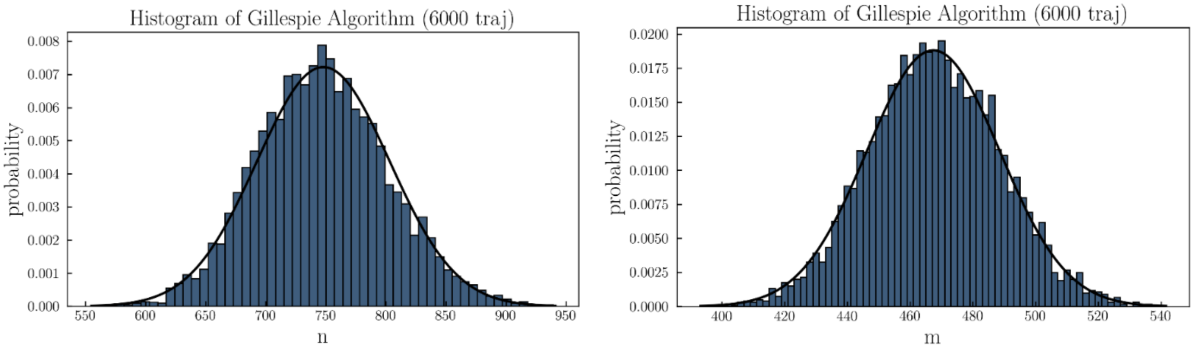


FIG. S4. Long-time distributions of $n$ and $m$. Histograms of the distribution of products $n$ (left panel) and $m$ (right panel) from a Gillespie simulation of Model 2 with 6000 trajectories. The black curve is a plot of our choice of Normal distribution with mean and variance derived from the generating functions (Section A).

# Section F: Bayesian framework, effects of the prior

The breakdown of the MLE for $n > k_p t$ can be regularized by including a prior estimate on $x$ which forces the probability of unphysically large $x$ to be very small. A simple choice is the exponential distribution $\text{Prior}(x) = \lambda e^{-\lambda x}$ where $\lambda$ determines the preference to estimate small $x$. The peak of the updated likelihood (i.e. the posterior) must then be found numerically. As seen below (Fig. S5), the additional information provided by the prior makes the estimation well-behaved across the boundary $n = k_p t$.

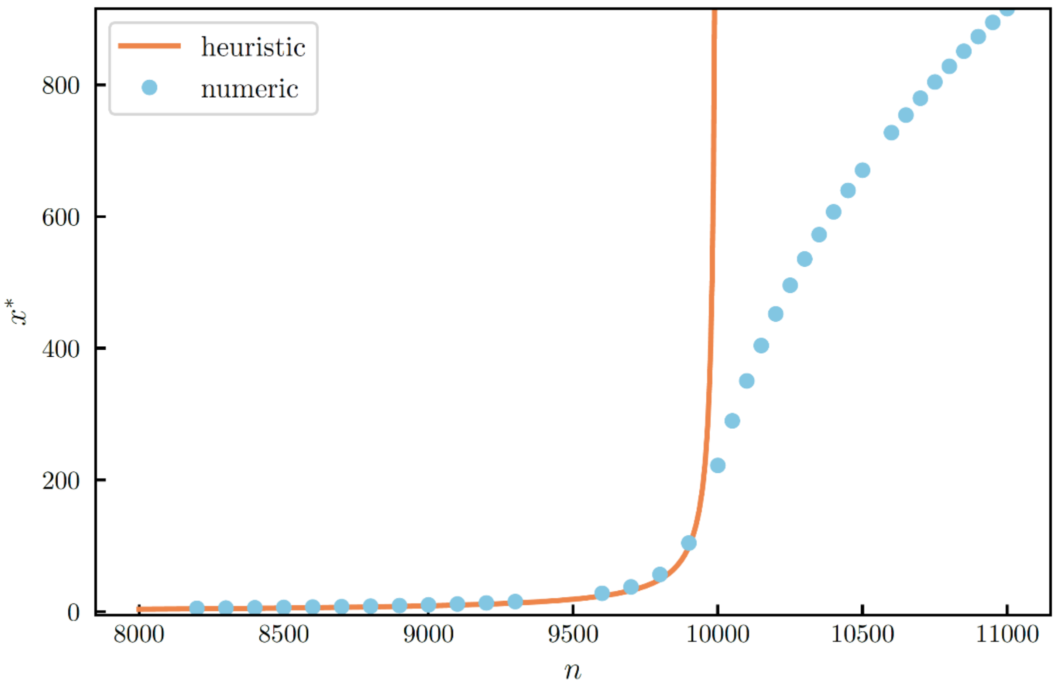


FIG. S5. Estimation with prior. The orange line shows the heuristic formula for the MLE, as already shown in Section A. The blue dots show the new MLE obtained by finding the peak of the likelihood function updated by a weakly informative exponential prior. The numerical MLE agrees very closely with the already validated estimates for low $n$ and moves smoothly across the $n = k_p t$ boundary. Parameters: $\lambda = 10^{-3}$, $k_p t = 10^4$, $k_{\mathrm{off}}/k_{\mathrm{on}} = 10^{-7}$. The value of $c$ was estimated and converted to $x^*$ using known $K_D = k_{\mathrm{off}}/k_{\mathrm{on}}$.
